# Supplementary material for: Handbook of LHC Higgs Cross Sections: 2. Differential Distributions
Source: arXiv:1201.3084 source file (2012-01-15)
Supplement: Supplementary file 1 [file SM4EW_tab.tex]

\begin{table}
\begin{center}
\caption[]{\label{tab:EWNLO}{NLO EW corrections to 
$\Pg\Pg\to \PH+X$ cross sections.}}
\begin{tabular}{rrrrrr}
\hline
$\MH[\UGeVZ]$ & $\delta$ [\%] & 
$\MH[\UGeVZ]$ & $\delta$ [\%] & 
$\MH[\UGeVZ]$ & $\delta$ [\%] \\
\hline
$100$ & $12.28$ & $120$ & $12.12$ & $140$ & $11.78$ \\
$150$ & $11.39$ & $160$ & $10.11$ & $180$ & $8.48$ \\
$190$ & $8.06$ & $200$ & $7.47$ & $250$ & $5.81$ \\
$300$ & $4.54$ & $400$ & $3.26$ & $500$ & ${-}2.54$ \\
$600$ & ${-}12.70$ & $700$ & ${-}24.90$ & $800$ & ${-}37.79$ \\
$900$ & ${-}50.77$ & $1000$ & ${-}64.19$ & $1100$ & ${-}80.84$ \\
\hline
\end{tabular}
\end{center}
\end{table}
