# Supplementary material for: Handbook of LHC Higgs Cross Sections: 2. Differential Distributions
Source: arXiv:1201.3084 source file (2012-01-15)
Supplement: Supplementary file 2 [file br_ff3.tex]

\begin{tabular}{ccccccc}
\hline  $\vphantom{\bar{\bar{\bar{\PQb}}}}$%
$\MH$ [GeV]&   $\Hbb$ & $\Htautau$ & $\Hmumu$ &   $\Hss$ &   $\Hcc$ &   $\Htt$ \\ \hline
347.0 & $1.83\cdot 10^{-3}$ & $1.49\cdot 10^{-4}$ & $5.15\cdot 10^{-7}$ & $4.79\cdot 10^{-7}$ & $5.65\cdot 10^{-5}$ & $1.93\cdot 10^{-2}$ \\
347.5 & $1.83\cdot 10^{-3}$ & $1.48\cdot 10^{-4}$ & $5.14\cdot 10^{-7}$ & $4.77\cdot 10^{-7}$ & $5.63\cdot 10^{-5}$ & $2.28\cdot 10^{-2}$ \\
348.0 & $1.80\cdot 10^{-3}$ & $1.46\cdot 10^{-4}$ & $5.07\cdot 10^{-7}$ & $4.71\cdot 10^{-7}$ & $5.56\cdot 10^{-5}$ & $2.66\cdot 10^{-2}$ \\
348.5 & $1.79\cdot 10^{-3}$ & $1.46\cdot 10^{-4}$ & $5.05\cdot 10^{-7}$ & $4.69\cdot 10^{-7}$ & $5.53\cdot 10^{-5}$ & $3.12\cdot 10^{-2}$ \\
349.0 & $1.77\cdot 10^{-3}$ & $1.43\cdot 10^{-4}$ & $4.97\cdot 10^{-7}$ & $4.62\cdot 10^{-7}$ & $5.45\cdot 10^{-5}$ & $3.58\cdot 10^{-2}$ \\
350.0 & $1.73\cdot 10^{-3}$ & $1.41\cdot 10^{-4}$ & $4.87\cdot 10^{-7}$ & $4.52\cdot 10^{-7}$ & $5.34\cdot 10^{-5}$ & $4.60\cdot 10^{-2}$ \\
351.0 & $1.70\cdot 10^{-3}$ & $1.38\cdot 10^{-4}$ & $4.78\cdot 10^{-7}$ & $4.43\cdot 10^{-7}$ & $5.23\cdot 10^{-5}$ & $5.61\cdot 10^{-2}$ \\
352.0 & $1.66\cdot 10^{-3}$ & $1.35\cdot 10^{-4}$ & $4.69\cdot 10^{-7}$ & $4.35\cdot 10^{-7}$ & $5.13\cdot 10^{-5}$ & $6.61\cdot 10^{-2}$ \\
353.0 & $1.63\cdot 10^{-3}$ & $1.33\cdot 10^{-4}$ & $4.60\cdot 10^{-7}$ & $4.26\cdot 10^{-7}$ & $5.03\cdot 10^{-5}$ & $7.61\cdot 10^{-2}$ \\
354.0 & $1.60\cdot 10^{-3}$ & $1.30\cdot 10^{-4}$ & $4.51\cdot 10^{-7}$ & $4.18\cdot 10^{-7}$ & $4.93\cdot 10^{-5}$ & $8.59\cdot 10^{-2}$ \\
355.0 & $1.56\cdot 10^{-3}$ & $1.27\cdot 10^{-4}$ & $4.42\cdot 10^{-7}$ & $4.09\cdot 10^{-7}$ & $4.83\cdot 10^{-5}$ & $9.55\cdot 10^{-2}$ \\
360.0 & $1.42\cdot 10^{-3}$ & $1.16\cdot 10^{-4}$ & $4.00\cdot 10^{-7}$ & $3.70\cdot 10^{-7}$ & $4.36\cdot 10^{-5}$ & $1.40\cdot 10^{-1}$ \\
370.0 & $1.18\cdot 10^{-3}$ & $9.67\cdot 10^{-5}$ & $3.35\cdot 10^{-7}$ & $3.08\cdot 10^{-7}$ & $3.64\cdot 10^{-5}$ & $2.14\cdot 10^{-1}$ \\
375.0 & $1.09\cdot 10^{-3}$ & $8.92\cdot 10^{-5}$ & $3.09\cdot 10^{-7}$ & $2.84\cdot 10^{-7}$ & $3.34\cdot 10^{-5}$ & $2.43\cdot 10^{-1}$ \\
380.0 & $1.00\cdot 10^{-3}$ & $8.28\cdot 10^{-5}$ & $2.87\cdot 10^{-7}$ & $2.62\cdot 10^{-7}$ & $3.10\cdot 10^{-5}$ & $2.67\cdot 10^{-1}$ \\
390.0 & $8.75\cdot 10^{-4}$ & $7.24\cdot 10^{-5}$ & $2.51\cdot 10^{-7}$ & $2.29\cdot 10^{-7}$ & $2.70\cdot 10^{-5}$ & $3.07\cdot 10^{-1}$ \\
400.0 & $7.75\cdot 10^{-4}$ & $6.44\cdot 10^{-5}$ & $2.23\cdot 10^{-7}$ & $2.02\cdot 10^{-7}$ & $2.39\cdot 10^{-5}$ & $3.36\cdot 10^{-1}$ \\
410.0 & $6.95\cdot 10^{-4}$ & $5.80\cdot 10^{-5}$ & $2.01\cdot 10^{-7}$ & $1.81\cdot 10^{-7}$ & $2.14\cdot 10^{-5}$ & $3.57\cdot 10^{-1}$ \\
420.0 & $6.31\cdot 10^{-4}$ & $5.28\cdot 10^{-5}$ & $1.83\cdot 10^{-7}$ & $1.65\cdot 10^{-7}$ & $1.94\cdot 10^{-5}$ & $3.72\cdot 10^{-1}$ \\
430.0 & $5.79\cdot 10^{-4}$ & $4.87\cdot 10^{-5}$ & $1.69\cdot 10^{-7}$ & $1.51\cdot 10^{-7}$ & $1.78\cdot 10^{-5}$ & $3.84\cdot 10^{-1}$ \\
440.0 & $5.35\cdot 10^{-4}$ & $4.51\cdot 10^{-5}$ & $1.56\cdot 10^{-7}$ & $1.40\cdot 10^{-7}$ & $1.65\cdot 10^{-5}$ & $3.92\cdot 10^{-1}$ \\
450.0 & $4.98\cdot 10^{-4}$ & $4.21\cdot 10^{-5}$ & $1.46\cdot 10^{-7}$ & $1.30\cdot 10^{-7}$ & $1.53\cdot 10^{-5}$ & $3.98\cdot 10^{-1}$ \\
460.0 & $4.66\cdot 10^{-4}$ & $3.96\cdot 10^{-5}$ & $1.37\cdot 10^{-7}$ & $1.21\cdot 10^{-7}$ & $1.43\cdot 10^{-5}$ & $4.02\cdot 10^{-1}$ \\
470.0 & $4.38\cdot 10^{-4}$ & $3.73\cdot 10^{-5}$ & $1.29\cdot 10^{-7}$ & $1.14\cdot 10^{-7}$ & $1.35\cdot 10^{-5}$ & $4.04\cdot 10^{-1}$ \\
480.0 & $4.14\cdot 10^{-4}$ & $3.54\cdot 10^{-5}$ & $1.23\cdot 10^{-7}$ & $1.08\cdot 10^{-7}$ & $1.27\cdot 10^{-5}$ & $4.04\cdot 10^{-1}$ \\
490.0 & $3.92\cdot 10^{-4}$ & $3.36\cdot 10^{-5}$ & $1.16\cdot 10^{-7}$ & $1.02\cdot 10^{-7}$ & $1.20\cdot 10^{-5}$ & $4.04\cdot 10^{-1}$ \\
500.0 & $3.72\cdot 10^{-4}$ & $3.20\cdot 10^{-5}$ & $1.11\cdot 10^{-7}$ & $9.70\cdot 10^{-8}$ & $1.14\cdot 10^{-5}$ & $4.03\cdot 10^{-1}$ \\
550.0 & $2.99\cdot 10^{-4}$ & $2.61\cdot 10^{-5}$ & $9.04\cdot 10^{-8}$ & $7.78\cdot 10^{-8}$ & $9.18\cdot 10^{-6}$ & $3.88\cdot 10^{-1}$ \\
600.0 & $2.49\cdot 10^{-4}$ & $2.20\cdot 10^{-5}$ & $7.64\cdot 10^{-8}$ & $6.48\cdot 10^{-8}$ & $7.64\cdot 10^{-6}$ & $3.64\cdot 10^{-1}$ \\
650.0 & $2.12\cdot 10^{-4}$ & $1.90\cdot 10^{-5}$ & $6.58\cdot 10^{-8}$ & $5.51\cdot 10^{-8}$ & $6.49\cdot 10^{-6}$ & $3.37\cdot 10^{-1}$ \\
700.0 & $1.82\cdot 10^{-4}$ & $1.66\cdot 10^{-5}$ & $5.74\cdot 10^{-8}$ & $4.73\cdot 10^{-8}$ & $5.58\cdot 10^{-6}$ & $3.09\cdot 10^{-1}$ \\
750.0 & $1.58\cdot 10^{-4}$ & $1.45\cdot 10^{-5}$ & $5.04\cdot 10^{-8}$ & $4.10\cdot 10^{-8}$ & $4.84\cdot 10^{-6}$ & $2.81\cdot 10^{-1}$ \\
800.0 & $1.38\cdot 10^{-4}$ & $1.28\cdot 10^{-5}$ & $4.44\cdot 10^{-8}$ & $3.57\cdot 10^{-8}$ & $4.21\cdot 10^{-6}$ & $2.54\cdot 10^{-1}$ \\
1000.0 & $8.18\cdot 10^{-5}$ & $7.92\cdot 10^{-6}$ & $2.74\cdot 10^{-8}$ & $2.12\cdot 10^{-8}$ & $2.50\cdot 10^{-6}$ & $1.65\cdot 10^{-1}$ \\
\hline\end{tabular}
