# Supplementary material for: Handbook of LHC Higgs Cross Sections: 2. Differential Distributions
Source: arXiv:1201.3084 source file (2012-01-15)
Supplement: Supplementary file 3 [file br_h4f_comb3.tex]

\begin{tabular}{ccccccc}
\hline$\MH$ [GeV]&     $\PH \to 4\Pe$ & $\PH \to 2\Pe 2\PGm$ &     $\PH \to 4\Pl$ &     $\PH \to 4\Pq$ &  $\PH \to 2\Pl 2\Pq$ &     $\PH \to 4\Pf$ \\ \hline 
 347.0 & $2.97\cdot 10^{-4}$ & $6.00\cdot 10^{-4}$ & $8.85\cdot 10^{-2}$ & $4.68\cdot 10^{-1}$ & $4.09\cdot 10^{-1}$ & $9.65\cdot 10^{-1}$ \\
 347.5 & $2.96\cdot 10^{-4}$ & $5.97\cdot 10^{-4}$ & $8.82\cdot 10^{-2}$ & $4.66\cdot 10^{-1}$ & $4.07\cdot 10^{-1}$ & $9.61\cdot 10^{-1}$ \\
 348.0 & $2.95\cdot 10^{-4}$ & $5.95\cdot 10^{-4}$ & $8.79\cdot 10^{-2}$ & $4.64\cdot 10^{-1}$ & $4.05\cdot 10^{-1}$ & $9.57\cdot 10^{-1}$ \\
 348.5 & $2.93\cdot 10^{-4}$ & $5.92\cdot 10^{-4}$ & $8.75\cdot 10^{-2}$ & $4.62\cdot 10^{-1}$ & $4.03\cdot 10^{-1}$ & $9.53\cdot 10^{-1}$ \\
 349.0 & $2.92\cdot 10^{-4}$ & $5.89\cdot 10^{-4}$ & $8.71\cdot 10^{-2}$ & $4.60\cdot 10^{-1}$ & $4.01\cdot 10^{-1}$ & $9.48\cdot 10^{-1}$ \\
 350.0 & $2.89\cdot 10^{-4}$ & $5.83\cdot 10^{-4}$ & $8.62\cdot 10^{-2}$ & $4.55\cdot 10^{-1}$ & $3.97\cdot 10^{-1}$ & $9.38\cdot 10^{-1}$ \\
 351.0 & $2.86\cdot 10^{-4}$ & $5.73\cdot 10^{-4}$ & $8.53\cdot 10^{-2}$ & $4.50\cdot 10^{-1}$ & $3.93\cdot 10^{-1}$ & $9.28\cdot 10^{-1}$ \\
 352.0 & $2.83\cdot 10^{-4}$ & $5.67\cdot 10^{-4}$ & $8.45\cdot 10^{-2}$ & $4.45\cdot 10^{-1}$ & $3.89\cdot 10^{-1}$ & $9.18\cdot 10^{-1}$ \\
 353.0 & $2.81\cdot 10^{-4}$ & $5.62\cdot 10^{-4}$ & $8.36\cdot 10^{-2}$ & $4.40\cdot 10^{-1}$ & $3.85\cdot 10^{-1}$ & $9.08\cdot 10^{-1}$ \\
 354.0 & $2.78\cdot 10^{-4}$ & $5.56\cdot 10^{-4}$ & $8.25\cdot 10^{-2}$ & $4.36\cdot 10^{-1}$ & $3.81\cdot 10^{-1}$ & $8.99\cdot 10^{-1}$ \\
 355.0 & $2.75\cdot 10^{-4}$ & $5.50\cdot 10^{-4}$ & $8.17\cdot 10^{-2}$ & $4.31\cdot 10^{-1}$ & $3.77\cdot 10^{-1}$ & $8.90\cdot 10^{-1}$ \\
 360.0 & $2.62\cdot 10^{-4}$ & $5.24\cdot 10^{-4}$ & $7.78\cdot 10^{-2}$ & $4.09\cdot 10^{-1}$ & $3.58\cdot 10^{-1}$ & $8.46\cdot 10^{-1}$ \\
 370.0 & $2.41\cdot 10^{-4}$ & $4.81\cdot 10^{-4}$ & $7.14\cdot 10^{-2}$ & $3.74\cdot 10^{-1}$ & $3.28\cdot 10^{-1}$ & $7.74\cdot 10^{-1}$ \\
 375.0 & $2.33\cdot 10^{-4}$ & $4.65\cdot 10^{-4}$ & $6.88\cdot 10^{-2}$ & $3.60\cdot 10^{-1}$ & $3.16\cdot 10^{-1}$ & $7.45\cdot 10^{-1}$ \\
 380.0 & $2.25\cdot 10^{-4}$ & $4.51\cdot 10^{-4}$ & $6.66\cdot 10^{-2}$ & $3.49\cdot 10^{-1}$ & $3.06\cdot 10^{-1}$ & $7.21\cdot 10^{-1}$ \\
 390.0 & $2.14\cdot 10^{-4}$ & $4.29\cdot 10^{-4}$ & $6.32\cdot 10^{-2}$ & $3.30\cdot 10^{-1}$ & $2.90\cdot 10^{-1}$ & $6.83\cdot 10^{-1}$ \\
 400.0 & $2.06\cdot 10^{-4}$ & $4.13\cdot 10^{-4}$ & $6.06\cdot 10^{-2}$ & $3.16\cdot 10^{-1}$ & $2.78\cdot 10^{-1}$ & $6.54\cdot 10^{-1}$ \\
 410.0 & $2.01\cdot 10^{-4}$ & $4.01\cdot 10^{-4}$ & $5.89\cdot 10^{-2}$ & $3.06\cdot 10^{-1}$ & $2.70\cdot 10^{-1}$ & $6.34\cdot 10^{-1}$ \\
 420.0 & $1.97\cdot 10^{-4}$ & $3.93\cdot 10^{-4}$ & $5.75\cdot 10^{-2}$ & $2.99\cdot 10^{-1}$ & $2.63\cdot 10^{-1}$ & $6.19\cdot 10^{-1}$ \\
 430.0 & $1.95\cdot 10^{-4}$ & $3.88\cdot 10^{-4}$ & $5.66\cdot 10^{-2}$ & $2.93\cdot 10^{-1}$ & $2.58\cdot 10^{-1}$ & $6.08\cdot 10^{-1}$ \\
 440.0 & $1.93\cdot 10^{-4}$ & $3.85\cdot 10^{-4}$ & $5.59\cdot 10^{-2}$ & $2.89\cdot 10^{-1}$ & $2.55\cdot 10^{-1}$ & $6.00\cdot 10^{-1}$ \\
 450.0 & $1.92\cdot 10^{-4}$ & $3.83\cdot 10^{-4}$ & $5.54\cdot 10^{-2}$ & $2.87\cdot 10^{-1}$ & $2.53\cdot 10^{-1}$ & $5.95\cdot 10^{-1}$ \\
 460.0 & $1.92\cdot 10^{-4}$ & $3.83\cdot 10^{-4}$ & $5.51\cdot 10^{-2}$ & $2.85\cdot 10^{-1}$ & $2.51\cdot 10^{-1}$ & $5.91\cdot 10^{-1}$ \\
 470.0 & $1.93\cdot 10^{-4}$ & $3.84\cdot 10^{-4}$ & $5.49\cdot 10^{-2}$ & $2.84\cdot 10^{-1}$ & $2.51\cdot 10^{-1}$ & $5.90\cdot 10^{-1}$ \\
 480.0 & $1.93\cdot 10^{-4}$ & $3.87\cdot 10^{-4}$ & $5.50\cdot 10^{-2}$ & $2.84\cdot 10^{-1}$ & $2.51\cdot 10^{-1}$ & $5.89\cdot 10^{-1}$ \\
 490.0 & $1.94\cdot 10^{-4}$ & $3.89\cdot 10^{-4}$ & $5.50\cdot 10^{-2}$ & $2.84\cdot 10^{-1}$ & $2.51\cdot 10^{-1}$ & $5.90\cdot 10^{-1}$ \\
 500.0 & $1.95\cdot 10^{-4}$ & $3.91\cdot 10^{-4}$ & $5.52\cdot 10^{-2}$ & $2.85\cdot 10^{-1}$ & $2.52\cdot 10^{-1}$ & $5.92\cdot 10^{-1}$ \\
 550.0 & $2.03\cdot 10^{-4}$ & $4.09\cdot 10^{-4}$ & $5.67\cdot 10^{-2}$ & $2.92\cdot 10^{-1}$ & $2.59\cdot 10^{-1}$ & $6.08\cdot 10^{-1}$ \\
 600.0 & $2.14\cdot 10^{-4}$ & $4.30\cdot 10^{-4}$ & $5.91\cdot 10^{-2}$ & $3.04\cdot 10^{-1}$ & $2.69\cdot 10^{-1}$ & $6.32\cdot 10^{-1}$ \\
 650.0 & $2.26\cdot 10^{-4}$ & $4.53\cdot 10^{-4}$ & $6.18\cdot 10^{-2}$ & $3.17\cdot 10^{-1}$ & $2.81\cdot 10^{-1}$ & $6.60\cdot 10^{-1}$ \\
 700.0 & $2.37\cdot 10^{-4}$ & $4.78\cdot 10^{-4}$ & $6.46\cdot 10^{-2}$ & $3.30\cdot 10^{-1}$ & $2.93\cdot 10^{-1}$ & $6.89\cdot 10^{-1}$ \\
 750.0 & $2.49\cdot 10^{-4}$ & $5.01\cdot 10^{-4}$ & $6.74\cdot 10^{-2}$ & $3.44\cdot 10^{-1}$ & $3.06\cdot 10^{-1}$ & $7.17\cdot 10^{-1}$ \\
 800.0 & $2.60\cdot 10^{-4}$ & $5.24\cdot 10^{-4}$ & $7.02\cdot 10^{-2}$ & $3.57\cdot 10^{-1}$ & $3.17\cdot 10^{-1}$ & $7.44\cdot 10^{-1}$ \\
1000.0 & $2.98\cdot 10^{-4}$ & $5.99\cdot 10^{-4}$ & $7.96\cdot 10^{-2}$ & $3.98\cdot 10^{-1}$ & $3.57\cdot 10^{-1}$ & $8.34\cdot 10^{-1}$ \\
\hline\end{tabular}
