# Supplementary material for: Handbook of LHC Higgs Cross Sections: 2. Differential Distributions
Source: arXiv:1201.3084 source file (2012-01-15)
Supplement: Supplementary file 4 [file br_vv3.tex]

\begin{tabular}{ccccccc}
\hline$\MH$ [GeV]&   $\Hgg$ & $\Hgaga$ &  $\HZga$ &   $\HWW$ &   $\HZZ$ & $\Gamma_{\PH}$ [GeV] \\ \hline
347.0 & $1.40\cdot 10^{-2}$ & $3.42\cdot 10^{-5}$ & $1.11\cdot 10^{-4}$ & $6.67\cdot 10^{-1}$ & $2.97\cdot 10^{-1}$ & $4.82$ \\
347.5 & $1.41\cdot 10^{-2}$ & $3.42\cdot 10^{-5}$ & $1.11\cdot 10^{-4}$ & $6.64\cdot 10^{-1}$ & $2.96\cdot 10^{-1}$ & $4.84$ \\
348.0 & $1.40\cdot 10^{-2}$ & $3.38\cdot 10^{-5}$ & $1.09\cdot 10^{-4}$ & $6.62\cdot 10^{-1}$ & $2.95\cdot 10^{-1}$ & $4.92$ \\
348.5 & $1.40\cdot 10^{-2}$ & $3.38\cdot 10^{-5}$ & $1.09\cdot 10^{-4}$ & $6.59\cdot 10^{-1}$ & $2.94\cdot 10^{-1}$ & $4.94$ \\
349.0 & $1.39\cdot 10^{-2}$ & $3.34\cdot 10^{-5}$ & $1.07\cdot 10^{-4}$ & $6.55\cdot 10^{-1}$ & $2.92\cdot 10^{-1}$ & $5.02$ \\
350.0 & $1.38\cdot 10^{-2}$ & $3.28\cdot 10^{-5}$ & $1.05\cdot 10^{-4}$ & $6.49\cdot 10^{-1}$ & $2.89\cdot 10^{-1}$ & $5.14$ \\
351.0 & $1.36\cdot 10^{-2}$ & $3.23\cdot 10^{-5}$ & $1.03\cdot 10^{-4}$ & $6.42\cdot 10^{-1}$ & $2.86\cdot 10^{-1}$ & $5.26$ \\
352.0 & $1.35\cdot 10^{-2}$ & $3.17\cdot 10^{-5}$ & $1.01\cdot 10^{-4}$ & $6.36\cdot 10^{-1}$ & $2.82\cdot 10^{-1}$ & $5.38$ \\
353.0 & $1.34\cdot 10^{-2}$ & $3.12\cdot 10^{-5}$ & $9.85\cdot 10^{-5}$ & $6.29\cdot 10^{-1}$ & $2.78\cdot 10^{-1}$ & $5.50$ \\
354.0 & $1.33\cdot 10^{-2}$ & $3.06\cdot 10^{-5}$ & $9.64\cdot 10^{-5}$ & $6.23\cdot 10^{-1}$ & $2.75\cdot 10^{-1}$ & $5.62$ \\
355.0 & $1.31\cdot 10^{-2}$ & $3.01\cdot 10^{-5}$ & $9.44\cdot 10^{-5}$ & $6.17\cdot 10^{-1}$ & $2.72\cdot 10^{-1}$ & $5.75$ \\
360.0 & $1.25\cdot 10^{-2}$ & $2.75\cdot 10^{-5}$ & $8.50\cdot 10^{-5}$ & $5.86\cdot 10^{-1}$ & $2.59\cdot 10^{-1}$ & $6.44$ \\
370.0 & $1.14\cdot 10^{-2}$ & $2.31\cdot 10^{-5}$ & $7.00\cdot 10^{-5}$ & $5.36\cdot 10^{-1}$ & $2.38\cdot 10^{-1}$ & $7.91$ \\
375.0 & $1.09\cdot 10^{-2}$ & $2.13\cdot 10^{-5}$ & $6.39\cdot 10^{-5}$ & $5.16\cdot 10^{-1}$ & $2.29\cdot 10^{-1}$ & $8.69$ \\
380.0 & $1.04\cdot 10^{-2}$ & $1.97\cdot 10^{-5}$ & $5.88\cdot 10^{-5}$ & $4.99\cdot 10^{-1}$ & $2.22\cdot 10^{-1}$ & $9.49$ \\
390.0 & $9.60\cdot 10^{-3}$ & $1.71\cdot 10^{-5}$ & $5.04\cdot 10^{-5}$ & $4.72\cdot 10^{-1}$ & $2.11\cdot 10^{-1}$ & $1.11\cdot 10^{1}$ \\
400.0 & $8.94\cdot 10^{-3}$ & $1.51\cdot 10^{-5}$ & $4.38\cdot 10^{-5}$ & $4.51\cdot 10^{-1}$ & $2.03\cdot 10^{-1}$ & $1.29\cdot 10^{1}$ \\
410.0 & $8.37\cdot 10^{-3}$ & $1.35\cdot 10^{-5}$ & $3.86\cdot 10^{-5}$ & $4.38\cdot 10^{-1}$ & $1.96\cdot 10^{-1}$ & $1.47\cdot 10^{1}$ \\
420.0 & $7.88\cdot 10^{-3}$ & $1.21\cdot 10^{-5}$ & $3.45\cdot 10^{-5}$ & $4.26\cdot 10^{-1}$ & $1.92\cdot 10^{-1}$ & $1.65\cdot 10^{1}$ \\
430.0 & $7.44\cdot 10^{-3}$ & $1.11\cdot 10^{-5}$ & $3.11\cdot 10^{-5}$ & $4.18\cdot 10^{-1}$ & $1.90\cdot 10^{-1}$ & $1.83\cdot 10^{1}$ \\
440.0 & $7.06\cdot 10^{-3}$ & $1.01\cdot 10^{-5}$ & $2.82\cdot 10^{-5}$ & $4.12\cdot 10^{-1}$ & $1.88\cdot 10^{-1}$ & $2.02\cdot 10^{1}$ \\
450.0 & $6.70\cdot 10^{-3}$ & $9.37\cdot 10^{-6}$ & $2.57\cdot 10^{-5}$ & $4.08\cdot 10^{-1}$ & $1.87\cdot 10^{-1}$ & $2.22\cdot 10^{1}$ \\
460.0 & $6.38\cdot 10^{-3}$ & $8.71\cdot 10^{-6}$ & $2.37\cdot 10^{-5}$ & $4.05\cdot 10^{-1}$ & $1.86\cdot 10^{-1}$ & $2.41\cdot 10^{1}$ \\
470.0 & $6.09\cdot 10^{-3}$ & $8.14\cdot 10^{-6}$ & $2.19\cdot 10^{-5}$ & $4.03\cdot 10^{-1}$ & $1.86\cdot 10^{-1}$ & $2.62\cdot 10^{1}$ \\
480.0 & $5.82\cdot 10^{-3}$ & $7.65\cdot 10^{-6}$ & $2.03\cdot 10^{-5}$ & $4.02\cdot 10^{-1}$ & $1.88\cdot 10^{-1}$ & $2.82\cdot 10^{1}$ \\
490.0 & $5.59\cdot 10^{-3}$ & $7.21\cdot 10^{-6}$ & $1.89\cdot 10^{-5}$ & $4.02\cdot 10^{-1}$ & $1.88\cdot 10^{-1}$ & $3.03\cdot 10^{1}$ \\
500.0 & $5.36\cdot 10^{-3}$ & $6.83\cdot 10^{-6}$ & $1.76\cdot 10^{-5}$ & $4.02\cdot 10^{-1}$ & $1.89\cdot 10^{-1}$ & $3.25\cdot 10^{1}$ \\
550.0 & $4.41\cdot 10^{-3}$ & $5.44\cdot 10^{-6}$ & $1.30\cdot 10^{-5}$ & $4.11\cdot 10^{-1}$ & $1.97\cdot 10^{-1}$ & $4.40\cdot 10^{1}$ \\
600.0 & $3.67\cdot 10^{-3}$ & $4.59\cdot 10^{-6}$ & $1.01\cdot 10^{-5}$ & $4.25\cdot 10^{-1}$ & $2.07\cdot 10^{-1}$ & $5.69\cdot 10^{1}$ \\
650.0 & $3.09\cdot 10^{-3}$ & $4.04\cdot 10^{-6}$ & $8.02\cdot 10^{-6}$ & $4.42\cdot 10^{-1}$ & $2.18\cdot 10^{-1}$ & $7.17\cdot 10^{1}$ \\
700.0 & $2.58\cdot 10^{-3}$ & $3.66\cdot 10^{-6}$ & $6.52\cdot 10^{-6}$ & $4.60\cdot 10^{-1}$ & $2.29\cdot 10^{-1}$ & $8.87\cdot 10^{1}$ \\
750.0 & $2.19\cdot 10^{-3}$ & $3.40\cdot 10^{-6}$ & $5.38\cdot 10^{-6}$ & $4.78\cdot 10^{-1}$ & $2.39\cdot 10^{-1}$ & $1.08\cdot 10^{2}$ \\
800.0 & $1.85\cdot 10^{-3}$ & $3.23\cdot 10^{-6}$ & $4.50\cdot 10^{-6}$ & $4.96\cdot 10^{-1}$ & $2.49\cdot 10^{-1}$ & $1.31\cdot 10^{2}$ \\
1000.0 & $8.92\cdot 10^{-4}$ & $3.15\cdot 10^{-6}$ & $2.51\cdot 10^{-6}$ & $5.54\cdot 10^{-1}$ & $2.81\cdot 10^{-1}$ & $2.61\cdot 10^{2}$ \\
\hline\end{tabular}
